# Supplementary material for: Electric Field Control of the Verwey Transition and Induced Magnetoelectric Effect in Magnetite
Source: arXiv:1202.6460 source file (2012-02-29)
Supplement: Supplementary file 1 [file Supplemental_Material.pdf]

**Electric Field Control of the Verwey Transition and Induced Magnetoelectric Effect in Magnetite: Supplemental Material**

**Section 1: Electric Field Control in Large Area $Fe_3O_4$ Thin Film Devices**

A shadow mask is used to define a channel for magnetite deposition with dimensions of 4.2 mm wide and 9.0 mm in length, covering a large portion of the substrate. $Fe_3O_4$ is deposited through the shadow mask and onto the MgO(001) buffer layer for single crystal growth by reactive molecular beam epitaxy. The dielectric layer (PMMA/$Al_2O_3$/MgO) and top gate electrode (Pd/Ti) is then deposited onto the $Fe_3O_4$. The top gate electrode has a length of 4.5 mm producing a gating region of 4.2 mm × 4.5 mm in the center of the sample. Temperature dependent resistance is measured through standard 2-probe measurements and DC *I-V* curves are taken at each temperature step to determine resistance values. Figure S1 shows the temperature dependence of resistance for applied electric fields of -1.2 MV/cm ($V_G$ = -40 V, red), 0 MV/cm ($V_G$ = 0 V, black), +1.2 MV/cm ($V_G$ = +40 V, blue), with the red arrow corresponding to the Verwey temperature ($T_V$) for electric fields ±1.2 MV/cm and the black arrow for 0 MV/cm. For zero electric field, $T_V$ = 117 K. In general, 50 nm $Fe_3O_4$ films demonstrated equivalent Verwey transition temperatures regardless of channel geometry. With the application of either positive or negative field, we find $T_V$ increases to 123 K, giving a $\Delta T_V$ = +6 K, which is larger than the 210 μm wide channel device presented in the main text. As in the case of the 210 μm wide devices, the shift in $T_V$ depends primary on the magnitude of the applied electric field as opposed to its sign. Typical gate leakage for this sample is 10 nA at the maximum field.

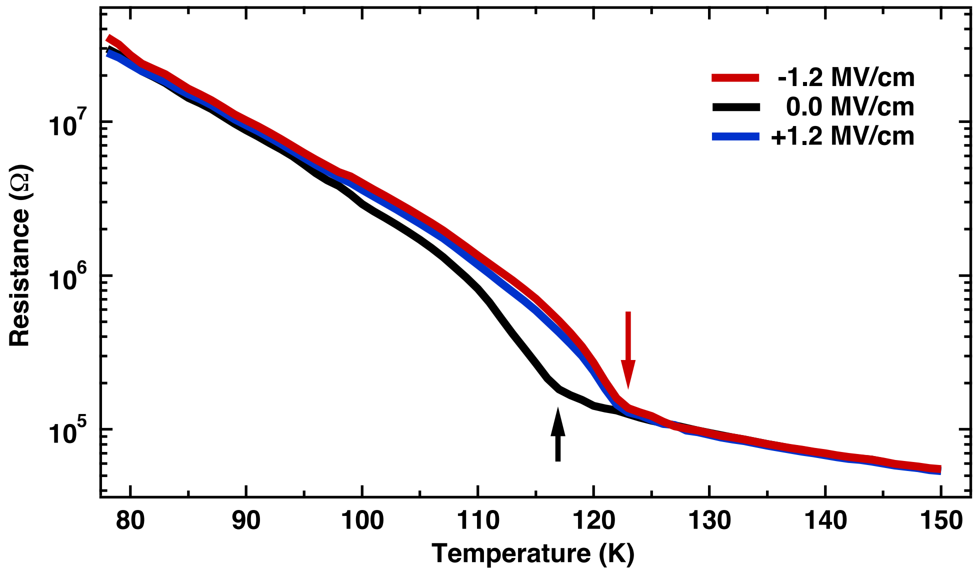


**Figure S1 Electric Field control of the Verwey transition for large area $Fe_3O_4$.** Temperature dependence of resistance for applied electric fields of +1.2 MV/cm (blue), 0 MV/cm (black), -1.2 MV/cm (red). The red arrow shows $T_V$ for electric fields of ± 1.2 MV/cm and the black arrow shows $T_V$ for electric field of 0 MV/cm, with $\Delta T_V$ = +6 K.

## Section 2: Magnetoelectric Coefficients for Various Materials

| Material | Type | $\lvert\alpha_{ME}\rvert$ (pT m/V) | Ref. |
|---|---|---|---|
| $Cr_2O_3$ | Single-Phase | 4.13 | [1],[2] |
| $Bi_5FeTi_3O_{15}$ | Single-Phase | 18.5 | [3] |
| $TbMn_2O_5$ | Single-Phase | 21 | [4] |
| $LiCoPO_4$ | Single-Phase | 30.6 | [5] |
| YIG | Single-Phase | ~30 | [5] |
| $BiFeO_3$-$CoFe_2O_4$ | Composite | 31.8 | [6] |
| $TbPO_4$ | Single-Phase | 36.7 | [5] |
| **$Fe_3O_4$** | **Single-Phase** | **585** | **this work** |
| $CoFe_2O_4$ / $BaTiO_3$ | Composite | 722 | [5] |
| LSMO / PZT | Composite | 6500 | [7] |
| PZT/Terfenol-D trilayer | Composite | 65040 | [8] |

## References


[1] X. He, Y. Wang, N. Wu, A. N. Caruso, E. Vescovo, K. D. Belashchenko, P. A. Dowben, and C. Binek, Nature Mater. **9**, 579 (2010).

[2] J. Ryu, S. Priya, K. Uchino, and H.-E. Kim, J. Electroceram. **8**, 107 (2002).

[3] S. Suryanarayana, Bull. Mater. Sci. **17**, 1259 (1994).

[4] N. Hur, S. Park, P. A. Sharma, J. S. Ahn, S. Guha, and S.-W. Cheong, Nature **429**, P392 (2004).

[5] M. Fiebig, J. Phys. D: Appl. Phys. **38**, R123 (2005).

[6] L. Yan, Z. Wang, Z. Xing, and J. Li, J. Appl. Phys. **107**, 064106 (2010).

[7] C. A. F. Vaz, J. Hoffman, Y. Segal, J. W. Reiner, R. D. Grober, Z. Zhang, C. H. Ahn, and F. J. Walker, Phys. Rev. Lett. **104**, 127202 (2010).

[8] J. Ryu, A. V. Carazo, K. Uchino, and H.-E. Kim, Jpn. J. Appl. Phys. **40**, 4948 (2001).
